# Supplementary material for: Learning Sim-to-Real Dense Object Descriptors for Robotic Manipulation
Source: arXiv:2304.08703 source file (2023-04-18)
Supplement: Supplementary file 1 [file Appendix.tex]

\appendix
\label{sec:appendix}
% \begin{center}
%     \textbf{APPENDIX}
%     %\textbf{Learning Sim-to-Real Dense Object Descriptors for Robotic Manipulation}
% \end{center}
\autoref{sec:supp_data_collection} is about the data used in this paper, and \autoref{sec:supp_srdons_results}, \autoref{sec:supp_grasping}, \autoref{sec:supp_picking} specify the experiments settings in more detail.
We also provided videos to demonstrate our experiment results, including matching object from sim-to-real with original object texture, finding matching points from sim-to-real with randomization texture, multiple point matching, object representation consistency in different scenes and view point, grasping objects, and two cases of picking cluttered objects.

\section{Data Collection}
\label{sec:supp_data_collection}
\begin{figure}[htb]
    \centering
    \begin{subfigure}[t]{0.3\columnwidth}
        \centering
        \frame{\includegraphics[width=\columnwidth]{Materials/graspnet_train_data_demo.png}}
        \caption{}
    \end{subfigure}
    \begin{subfigure}[t]{0.3\columnwidth}
        \centering
        \frame{\includegraphics[width=\columnwidth]{Materials/graspnet_test_data_demo.png}}
        \caption{}
    \end{subfigure}
    \begin{subfigure}[t]{0.3\columnwidth}
        \centering
        \frame{\includegraphics[width=\columnwidth]{Materials/novel_test_data_demo.png}}
        \caption{}
    \end{subfigure}
    
    \caption{Sample objects of different dataset. (a) Training dataset from GraspNet train split. (b) Testing dataset from GraspNet test split. (c) Testing dataset of novel household objects.}
    \label{fig:dataset}
\end{figure}

In the simulation, we use V-REP to generate the simulated data.
We captured 60 different scenes total, each scene contains 9-10 objects.
For a scene, we took 50 RGBD images with different view-pose and also record the 6D object poses and the camera parameters related to each images.
We apply texture and domain randomization in 30 scenes, and for the other 30 scenes, the objects maintain the original texture.
To apply randomization, we change the texture of the object and the background's color after every capturing steps. 
\autoref{fig:dataset} shows some objects from the GraspNet dataset (train and test splits), and novel household objects.

In the real data, we mainly use data from the GraspNet dataset.
We use 60 different scenes in total.
Each scene contains 9-10 objects, and they captured 256 RGBD images with the 6D object poses and the camera parameters related to each images.
However, to make the view of a scene sufficiently different, we sample less images per scene, namely 50 images per scene.
\autoref{fig:sample_images} shows examples of real and simulated images. 

\begin{figure}[htb]
    \centering
    \begin{subfigure}[t]{0.32\columnwidth}
        \centering
        \includegraphics[width=\columnwidth]{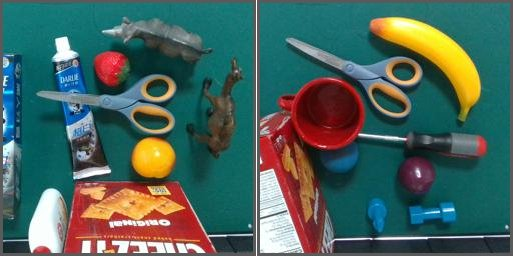}
        \caption{}
    \end{subfigure}
        \begin{subfigure}[t]{0.32\columnwidth}
        \centering
        \includegraphics[width=\columnwidth]{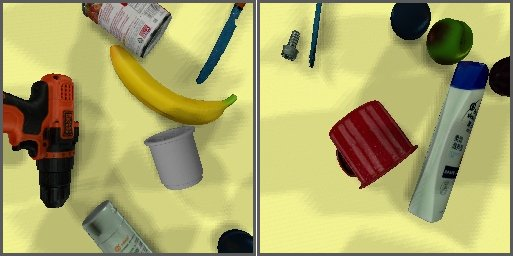}
        \caption{}
    \end{subfigure}
        \begin{subfigure}[t]{0.32\columnwidth}
        \centering
        \includegraphics[width=\columnwidth]{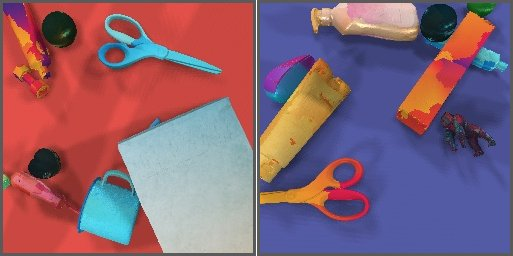}
        \caption{}
    \end{subfigure}
   
    \caption{Sample images from different data domains. (a) Real images from GraspNet. (b) Simulation images generated by V-REP. (c) Simulated images with texture and background randomization.}
    \label{fig:sample_images}
\end{figure}

%\section{Experiment Details}
%\label{sec:supp_experiment_details}
%In this Appendix, we specify the training parameters for our experiments described in Section %\ref{sec:experiments}, and provide more experimental results.

\section{SRDONs Training}
\label{sec:supp_srdons_results}

\begin{figure}[]
\begin{center}
  \includegraphics[width=0.8\columnwidth]{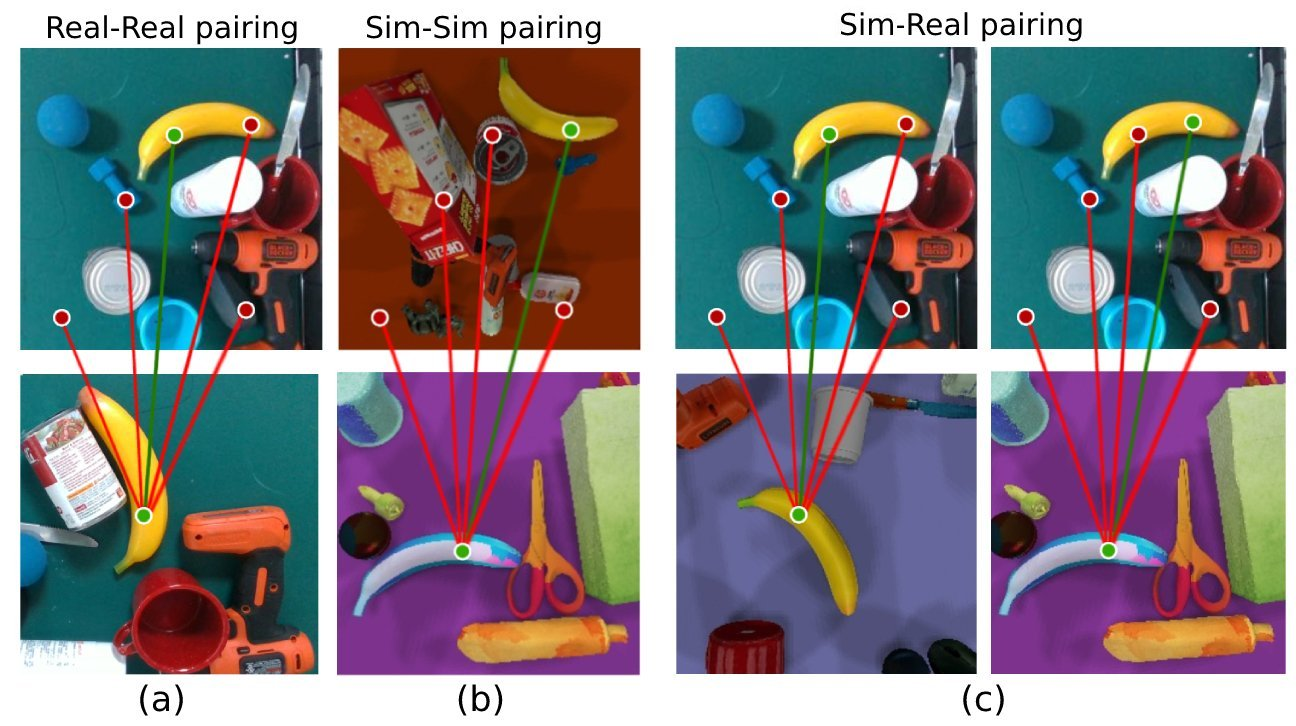}
  \caption{Different pairing type for training SRDONs. (a) Real-Real matching. (b) Sim-Sim matching. (c) Sim-Real matching. A pair of green dots indicate match-point; while a pair of red dots indicate non-match points.}
  \label{fig:mathcing_example}
\end{center}  
\end{figure}

\begin{figure}[t!]
    \centering
    \begin{subfigure}[t]{0.49\columnwidth}
        \includegraphics[width=\columnwidth]{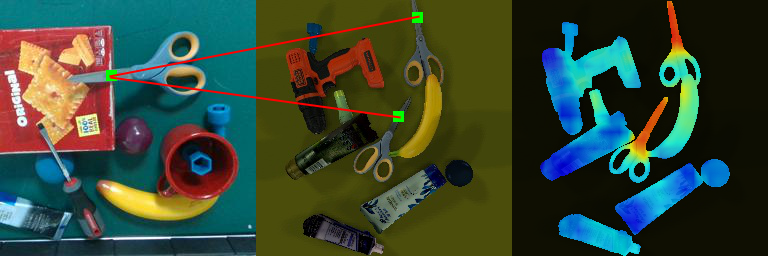}
        \caption{Multiple matching with original texture.}
        \label{fig:matchPoint}
    \end{subfigure}
    \begin{subfigure}[t]{0.49\columnwidth}
        \includegraphics[width=\columnwidth]{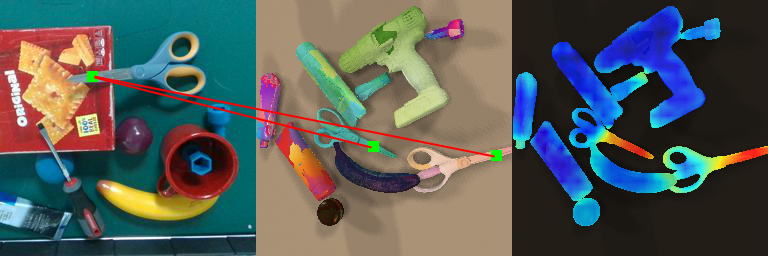}
        \caption{Multiple matching with object texture randomization.}
        \label{fig:objectNonMatchPoint}
    \end{subfigure}
    \caption{One to multiple objects matching evaluation. The heatmaps (in the right) indicate how much each pixel of the simulated images (in the middle) matches to the selected pixel in the real images (in the left). Note that red indicates better matching.}
    \label{fig:one_to_multiple_matching}
\end{figure}

\begin{figure}[t!]
    \centering
        \includegraphics[width=0.5\columnwidth]{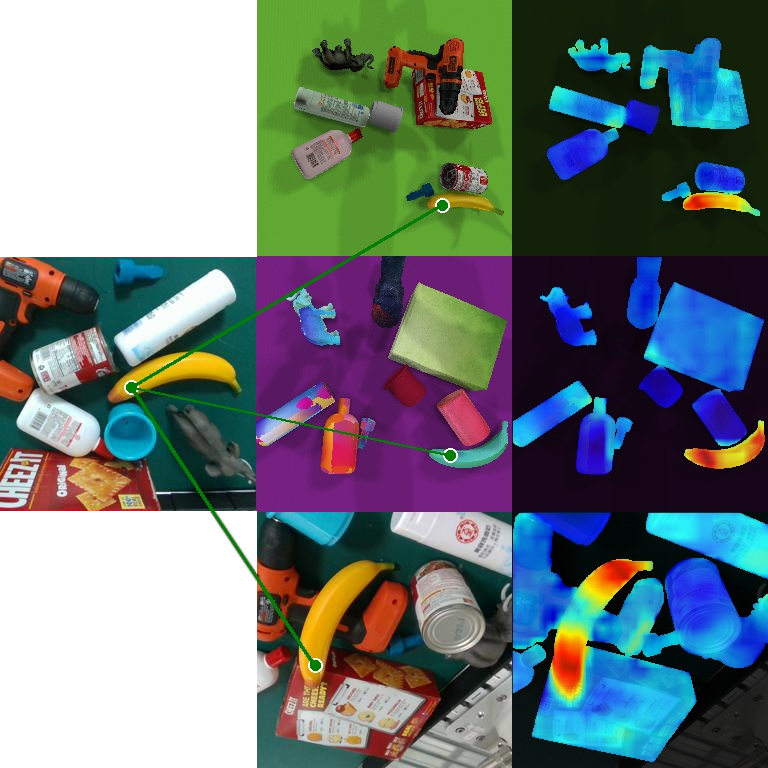}
    \caption{Matching result in different data domains. The image in the first column is the source (real) image with query point. The second column contains the target images with best-match point by the descriptors. Second row images from top to bottom: simulation image with original texture, simulation image with randomization, real image in different scene. The third column is the heatmaps indicate how much each pixel of the target images match to the query pixel in the source image. Note that red indicates better matching.}
    \label{fig:matching_different_domain}
\end{figure}

\begin{figure}[t!]
    \centering
        \includegraphics[width=0.6\columnwidth]{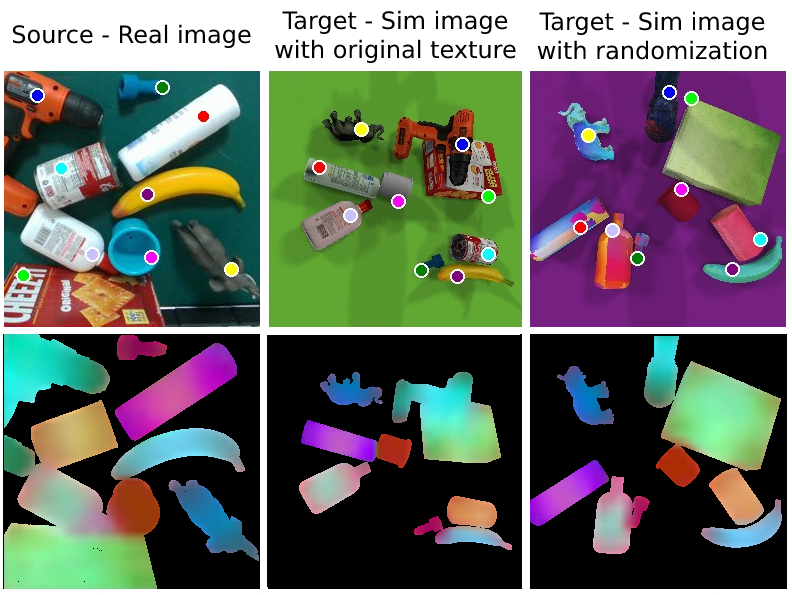}
    \caption{Multiple to multiple objects matching evaluation from simulation to real image. A pair of dots with the same color indicate the match point from the source image (real image, in the left) and the target images (simulation image with original text in the middle and simulation image with texture randomization in the right). The second row is the visualization of the descriptors with the above inputs.}
    \label{fig:multiple_to_multiple_matching}
\end{figure}

Similar to \cite{florencemanuelli2018dense}, we use 34-layers, stride-8 ResNet (ResNet34\_8s, pretrained on ImageNet) as the network structure for training our SRDONs.
For training, we use Adam optimizer with a learning rate of 0.0005 and a momentum of 0.9. The learning rate drops by 0.9 every 5000 steps.
We use 120k pairs of images, for each of which, we samples 1000 pairs of matching points, and 5000 pairs of non-matching points (object to object non-matching, object to background non-matching, background to background non-matching).

To select a pair of images, we uniformly sample pairing types (Sim-Sim, Real-Real, and Sim-Real). Once a type has been sampled, we then chose whether the two images are from the same scene or different scenes (with the probability of 30\%and 70\%, respectively).
For Sim-Real matching, two images come from different scenes, since they come from different data domains. \autoref{fig:mathcing_example} shows examples of different pairing types (Sim-Sim, Real-Real, and Sim-Real).
%\autoref{tab:sup_srdons_tranining_configuration} show the details of training configuration with different methods.

\autoref{fig:one_to_multiple_matching} demonstrates that our SRDONs matching result with one to multiple objects in different domains between simulated and real objects.
\autoref{fig:matching_different_domain} and \autoref{fig:multiple_to_multiple_matching} demonstrate the matching result in with multi-objects scenarios. Our SRDONs produces robust matching result in multiple objects scenarios with different data domains.
More experiment results will be shows in the supplementary videos.

% \todo[inline]{add more explanation from the IJCAI rebuttal}
% \todo[inline]{More evalutaion result and explantion}

\section{Grasping Objects}
\label{sec:supp_grasping}

\begin{figure}[]
\begin{center}
  \includegraphics[width=0.35\columnwidth]{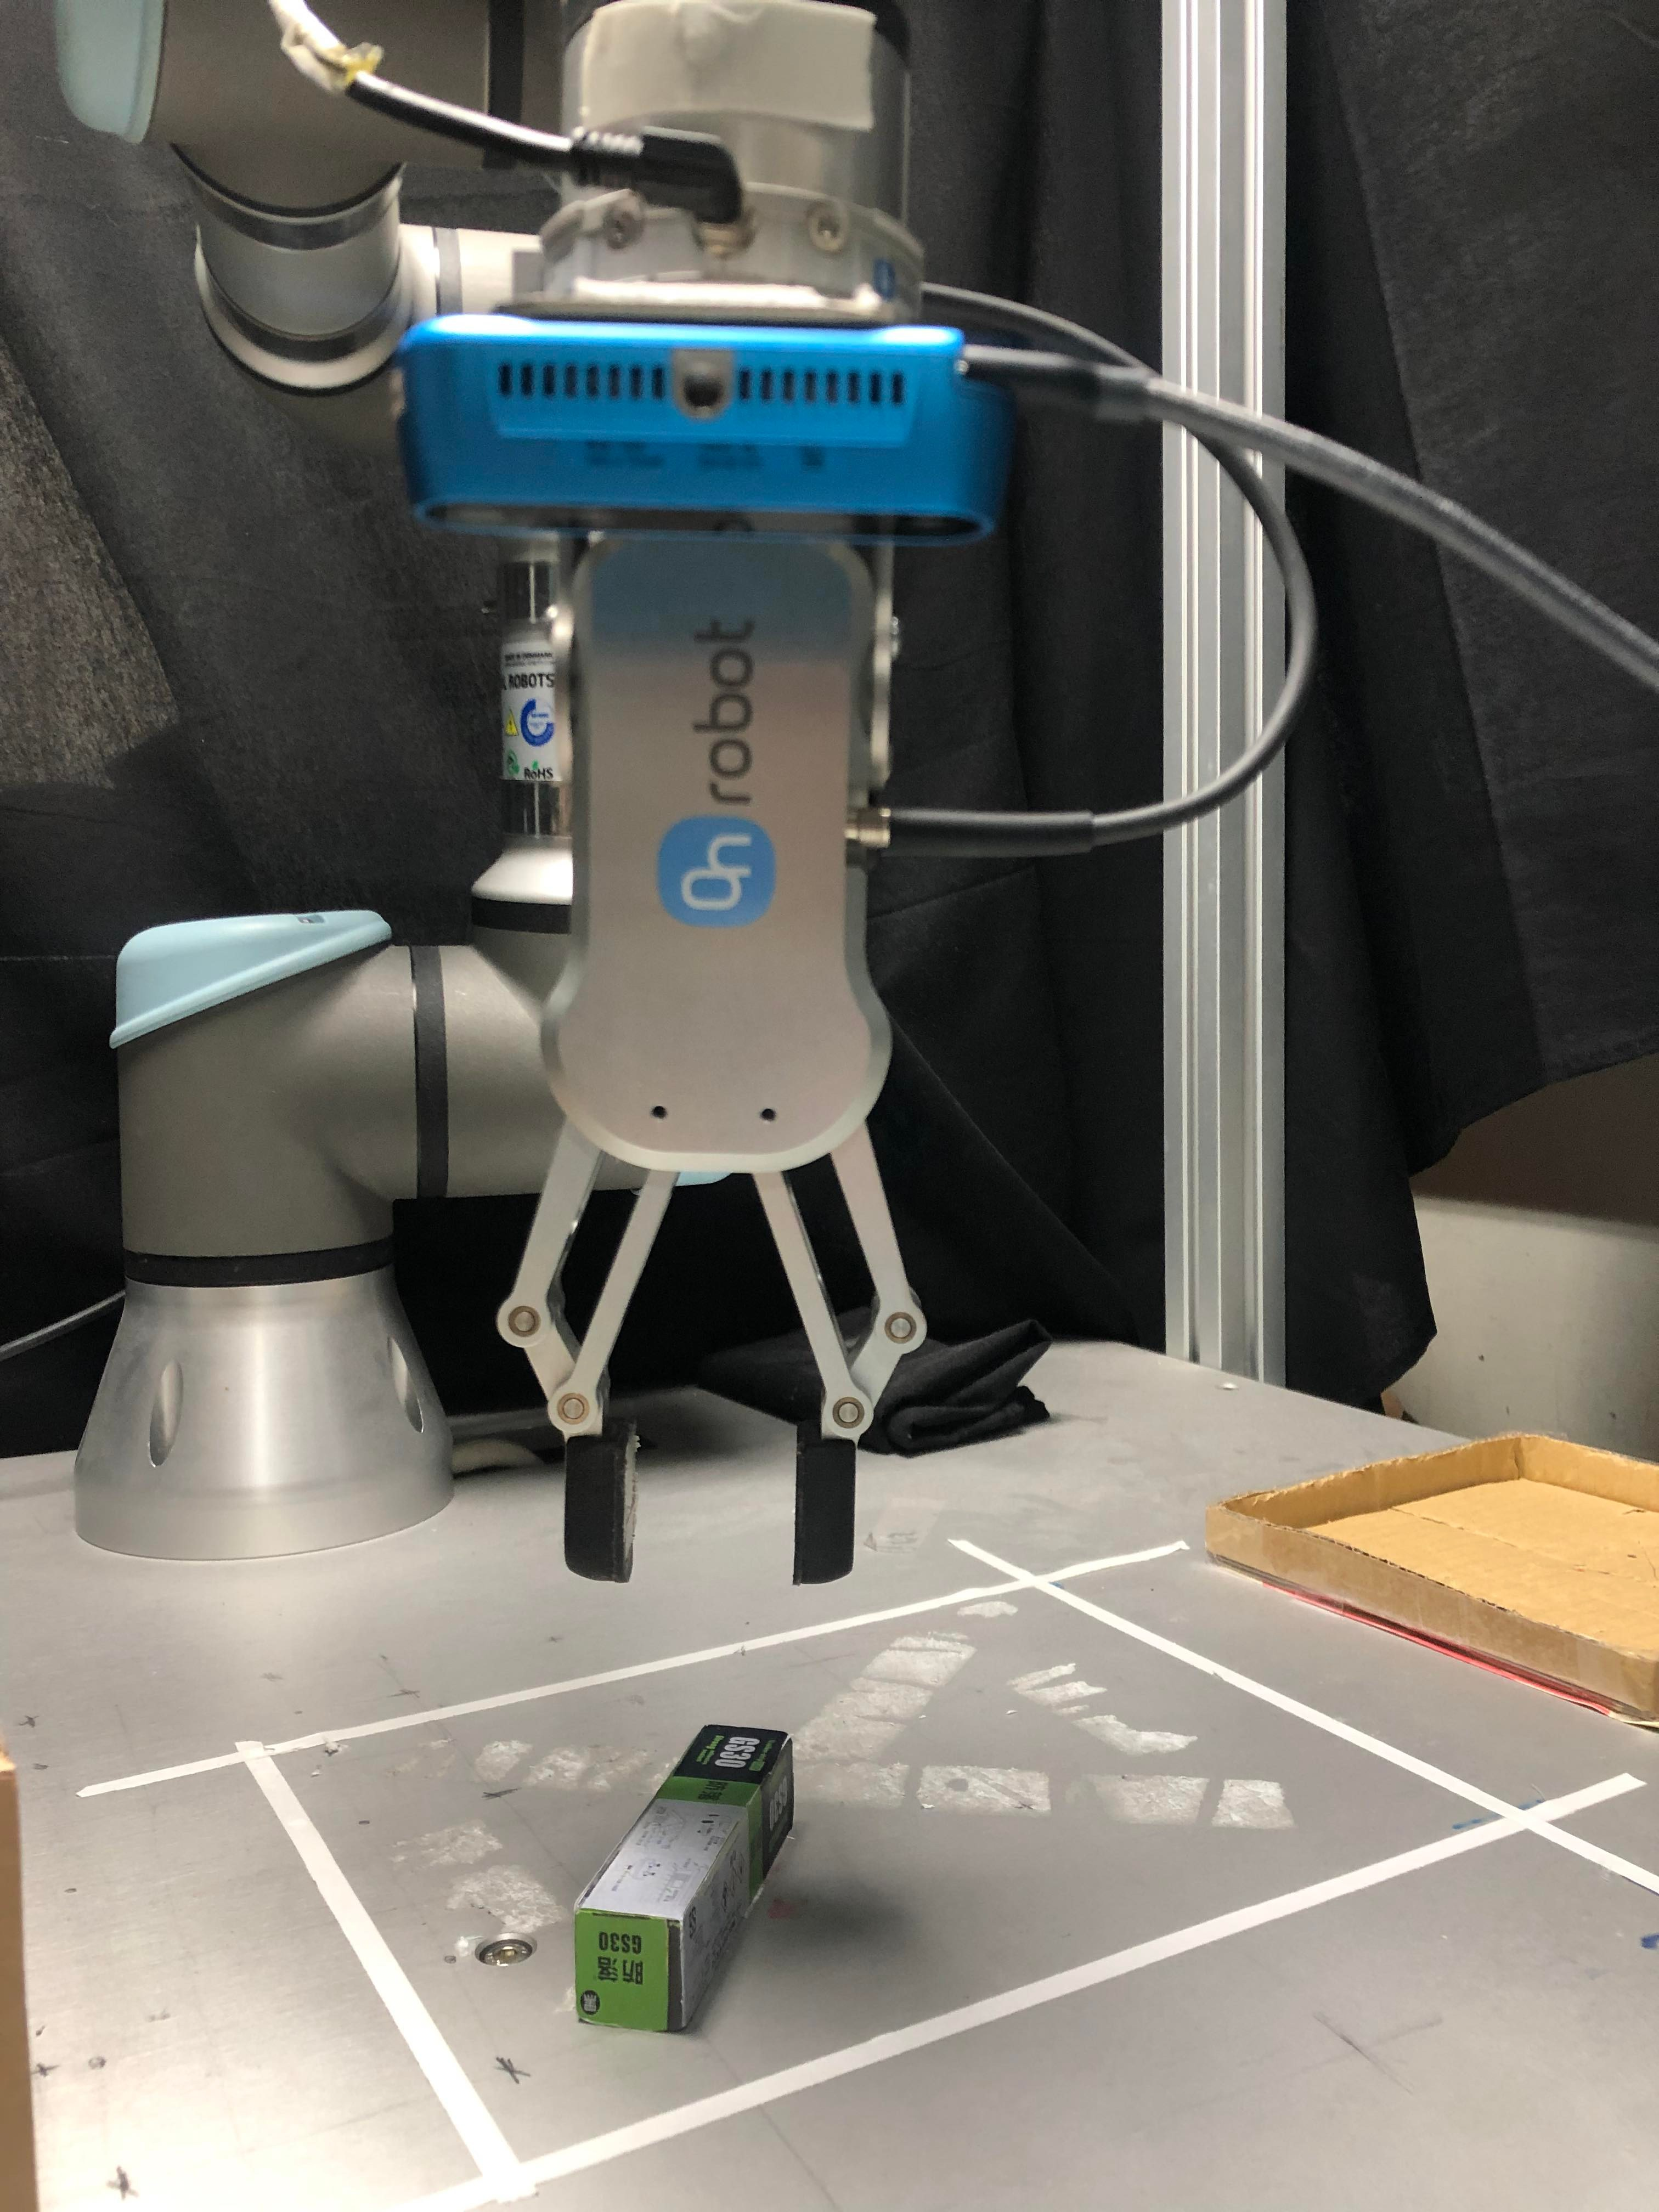}
  \caption{Real experiment setup for grasping objects. We use a UR-3 robot arm with a RG-2 gripper.}
  \label{fig:supp_real_grasp}
\end{center}  
\end{figure}

\begin{figure}[hbt!]
    \centering
    \begin{subfigure}{0.45\columnwidth}
        \centering
        \includegraphics[width=\columnwidth]{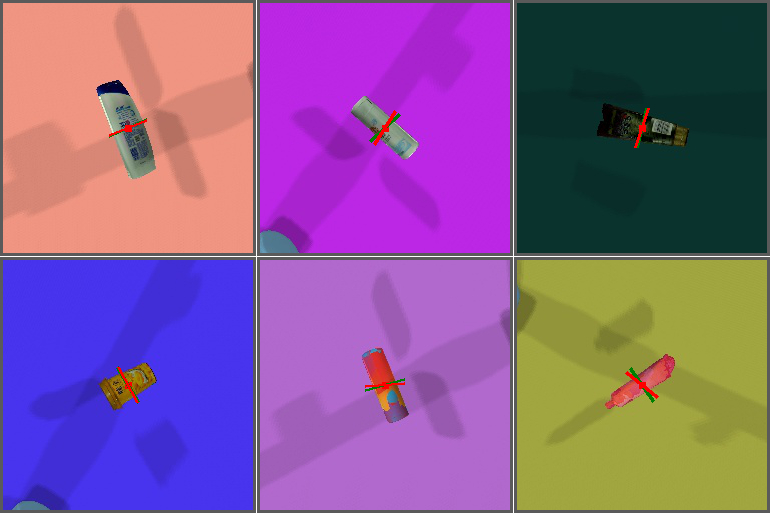}
        \caption{Grasping pose prediction in simulation.}
    \end{subfigure}
    \begin{subfigure}{0.45\columnwidth}
        \centering
        \includegraphics[width=\columnwidth]{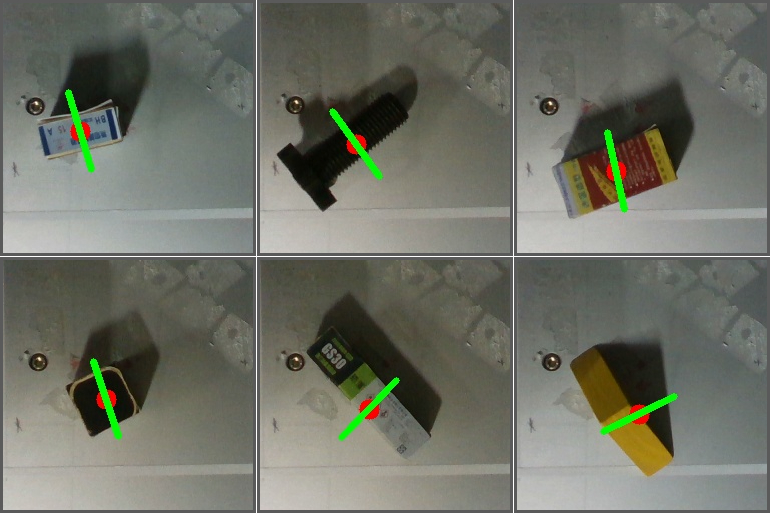}
        \caption{Grasping pose prediction with real objects.}
    \end{subfigure}
    \caption{Grasping object prediction. In the simulation, the green line is ground-truth pose; the red line is predicted pose. The center dots indicate the position to grasp the object. In real objects, there are only predicted grasping poses.}
    \label{fig:sup_grasping_result}
\end{figure}

\textbf{Hardware setup.} The RGBD observation (resolution 640x480) is captured by an Intel RealSense D435i, mounted on an UR-3 robot. \autoref{fig:supp_real_grasp} shows our setup in the real experiment for robot grasping object task.

\textbf{Network Structure.} For the network structure, as described in Subsection \ref{sec:policy_networ}, we modify the network from reinforcement learning to supervised learning.
We first remove the value head, and then replace the fully convolutional layers by fully connected layers, which return the predicted grasping pose with the position ($x$, $y$) and the z-orientation ($\theta$). Therefore, the output is ($x$, $y$,$\theta$) $\in \mathbb{R}^{3}$.

\textbf{Training Details.}
For training the supervised learning, we implement a mini-batch gradient descent version with python 3.8 and PyTorch.
We use the Adam optimizer with a learning rate of 0.001 and a momentum of 0.9. We train the network on single Nvidia GTX-1080 Ti and Xeon CPU at 2GHz.

\autoref{fig:sup_grasping_result} shows our prediction examples with the object in both simulation and real-world. We also provided the demonstration videos in the supplementary material.

\section{Picking Cluttered General Objects}
\label{sec:supp_picking}

\textbf{Network Structure.} \autoref{fig:sp_rl_network_structure} shows the network structure that we use in picking cluttered objects task.
We have two streams of ResNet34\_8s blocks, one of which is the pre-trained SRDONs network, the other is depth stream.
We then concatenate the corresponding output of ResNet blocks, and feed them through a U-Net like structure.
The SRDONs stream is frozen during RL training.
At the bottle-neck of U-Net, we add few fully connected layers for the critic head of the Actor-Critic method.
The actor head returns the score map, indicate the position to pick the object, which is $O \in \mathbb{R}^{WxH} $.

\textbf{Training Details.} 
For the network architecture as described in Subsection \ref{sec:policy_networ}, we implemented PPO \cite{Schulman2017PPO}, an Actor-Critic with python 3.8 and PyTorch.
We use the Adam optimizer with a learning rate of 0.0005 and a momentum of 0.9.
Parameters specific for Actor-Critics are: entropy coefficients beta is 0.001, the clipping parameter epsilon is 0.2, and discount factor gamma is 0.3. 
We train the policy network with 4 parallel simulation environments on a single Nvidia GTX-1080 Ti and Xeon CPU at 2GHz.

The reward are set as follows: +0.1 for each successful picks, -0.1 for a failed pick, and -1 for terminal steps (except the completion).

An episode terminates upon the fulfillment of any of the following conditions.
\begin{inparaenum}[(a)]
    \item{All objects have been successfully picked.}
    \item{The number of actions exceeds twice of the number of objects at the beginning of the episode.}
    \item{The robot arm is uncontrollable or unsafe to operate with. For example, the robot arm collides with the basket, the table, or itself, and the robot arm controller fails.}
\end{inparaenum}

In the simulation environment, we train each method in the simulation with 10 objects sampled randomly from GraspNet train split. 
For testing, we ran 50 runs with 20 and 30 objects from GraspNet test splits, and novel household objects. 
Note that the testing scenarios are more cluttered than the training scenarios. 

After training in simulation, we directly evaluate the performance of the trained policy network in the real-world. 
In the real-world, we run 22 tests with a basket containing 10 novel household objects for each method.
\autoref{fig:sim_env_demo} and \autoref{fig:real_env_demo} show how we setup the simulation and the real environment for picking cluttered objects. We also provided the demonstration videos in the supplementary material.

\begin{figure}[t!]
        \centering
        \includegraphics[width=0.65\textwidth]{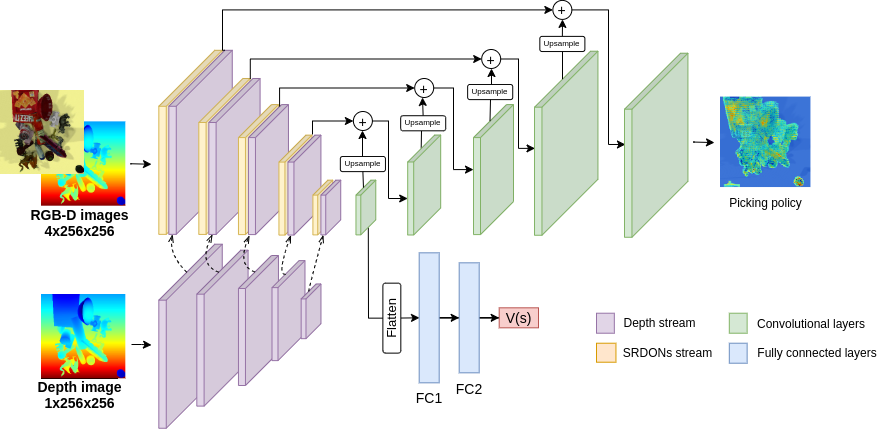}
        \caption{The network structure that combines SRDONs with depth stream in a U-Net fashion proposed by \cite{giang2021using}. The yellow boxes are the SRDONs stream; the pupple boxes are the depth stream; the green boxes are 2D convolution layers, which are connected in a U-Net fashion; blue boxes are fully connected layers, which return the critic in Actor-Critic.}
        \label{fig:sp_rl_network_structure}
\end{figure}

\begin{comment}
\begin{figure}[t!]
\begin{center}
  \includegraphics[width=0.5\columnwidth]{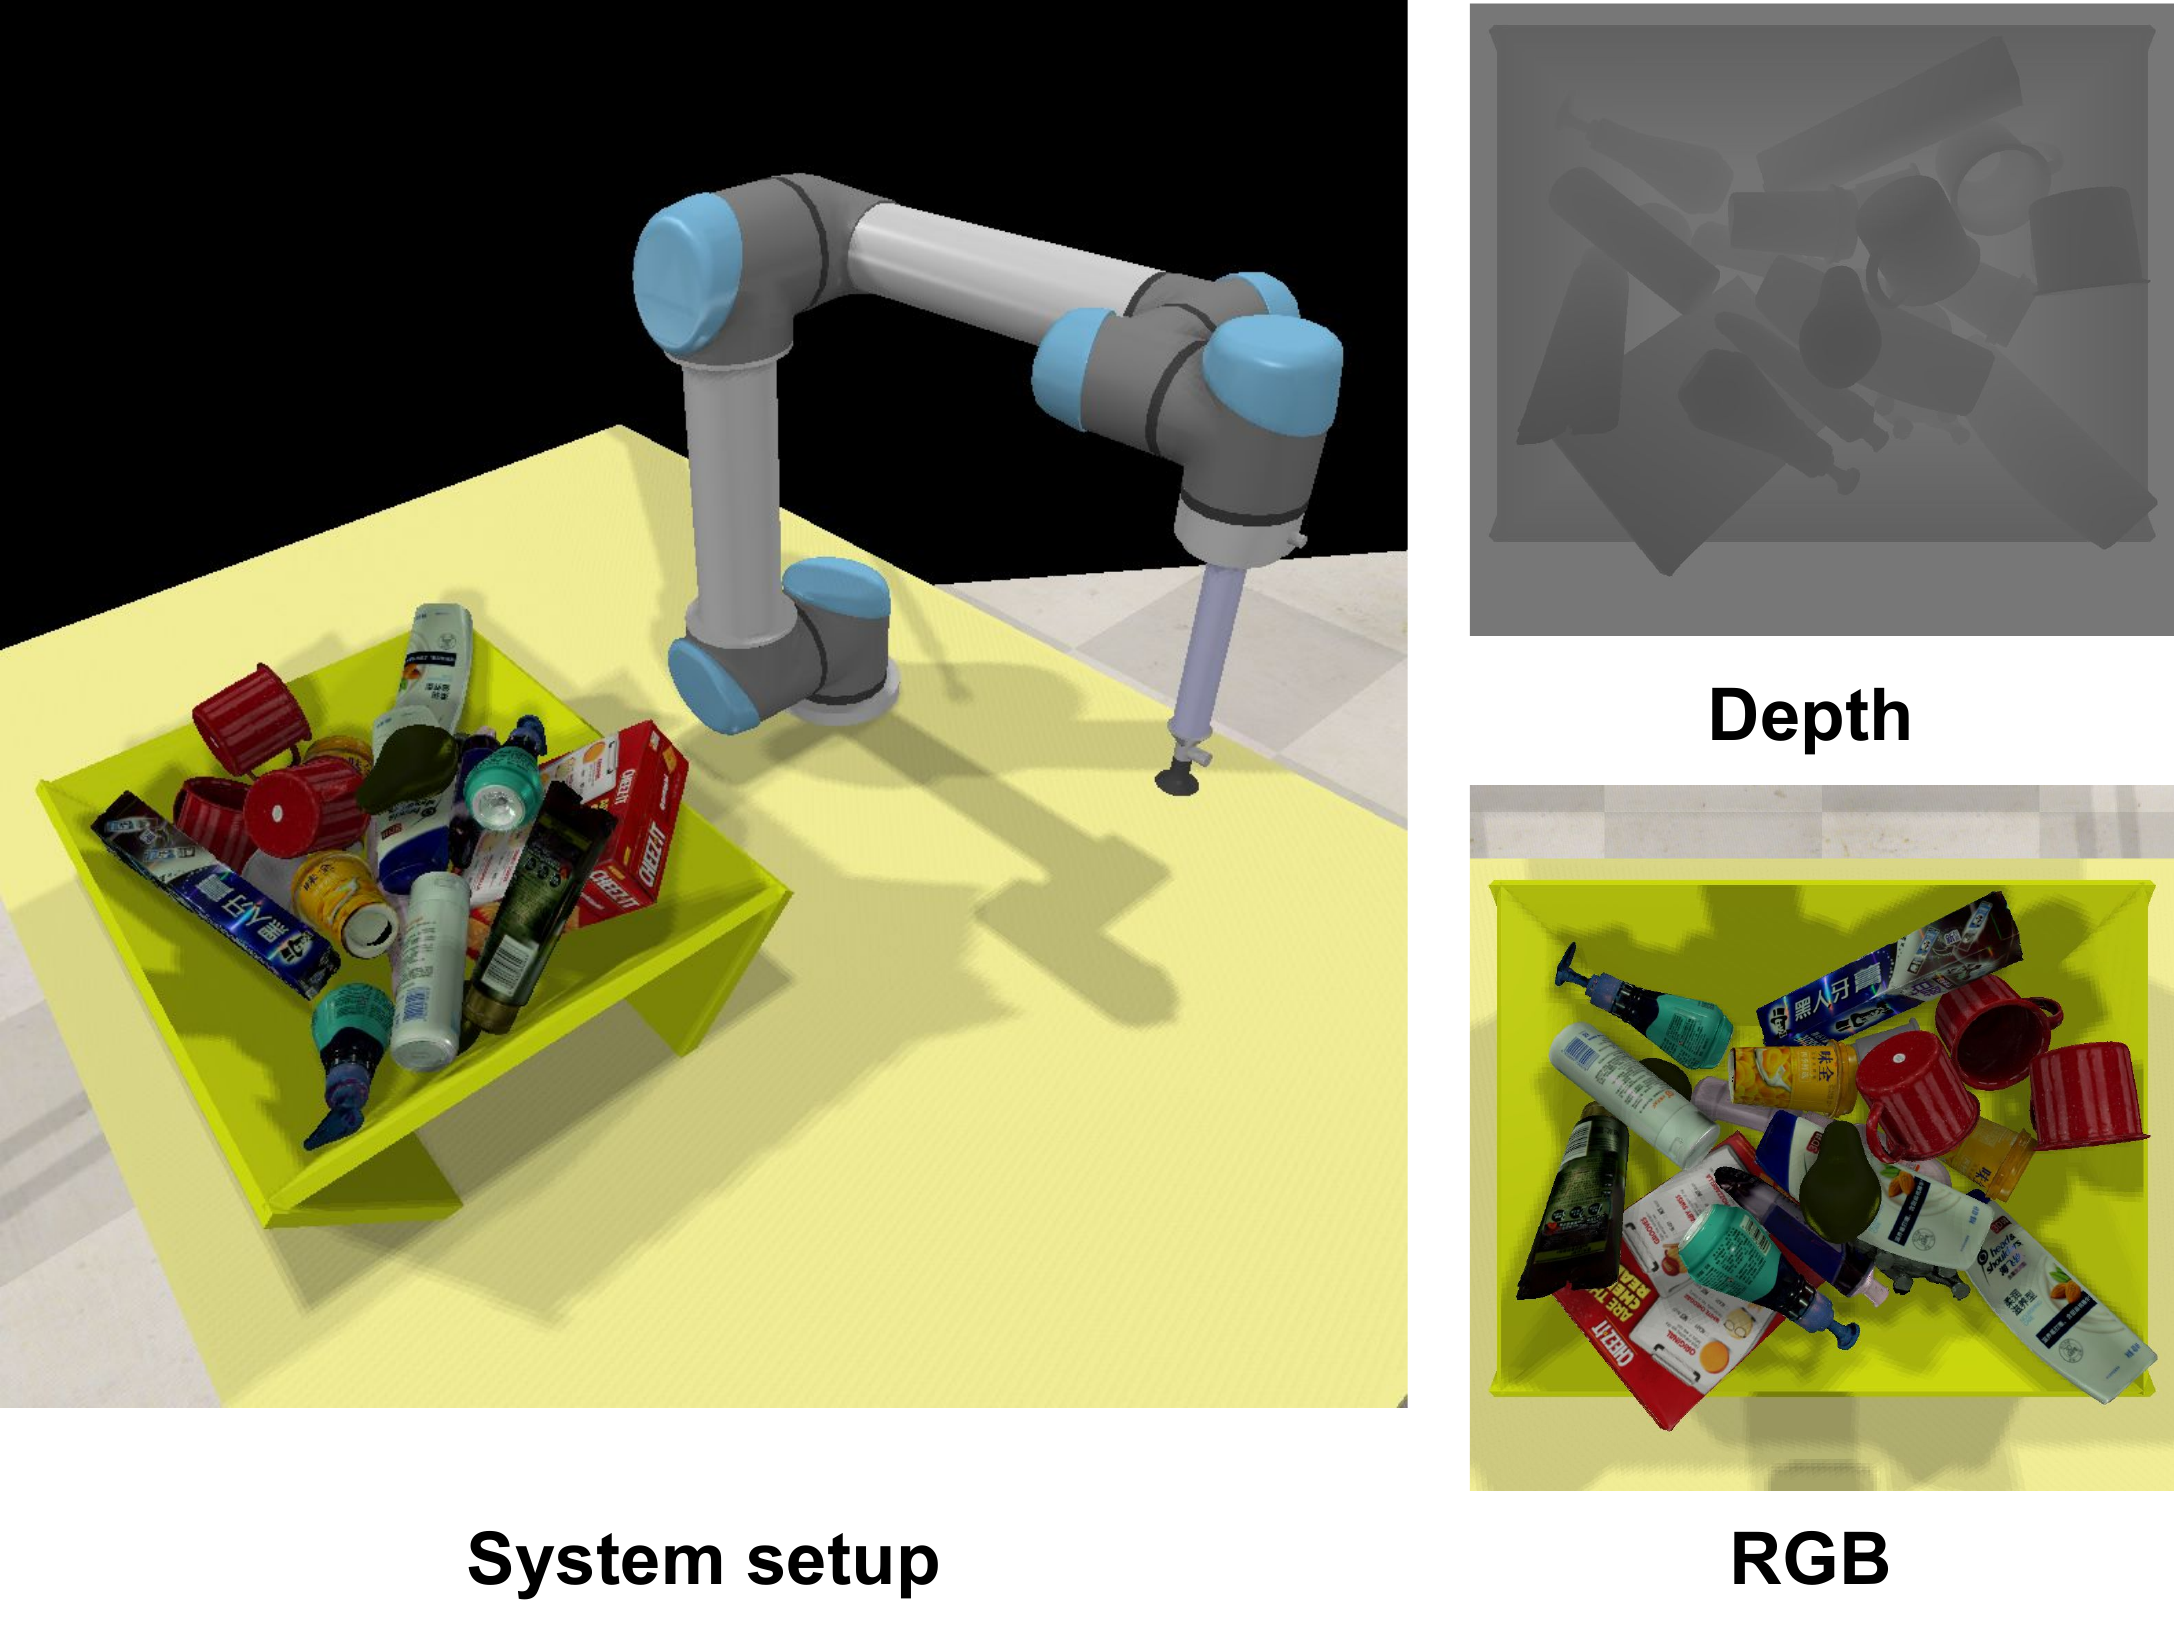}
  \caption{\textbf{Replace new image}The simulation picking system setup, and sample RGB and depth images. We use a UR-5 robot arm with a suction pad gripper.}
  \label{fig:sim_env_demo}
\end{center}  
\end{figure}

\begin{figure}[]
\begin{center}
  \includegraphics[width=0.5\columnwidth]{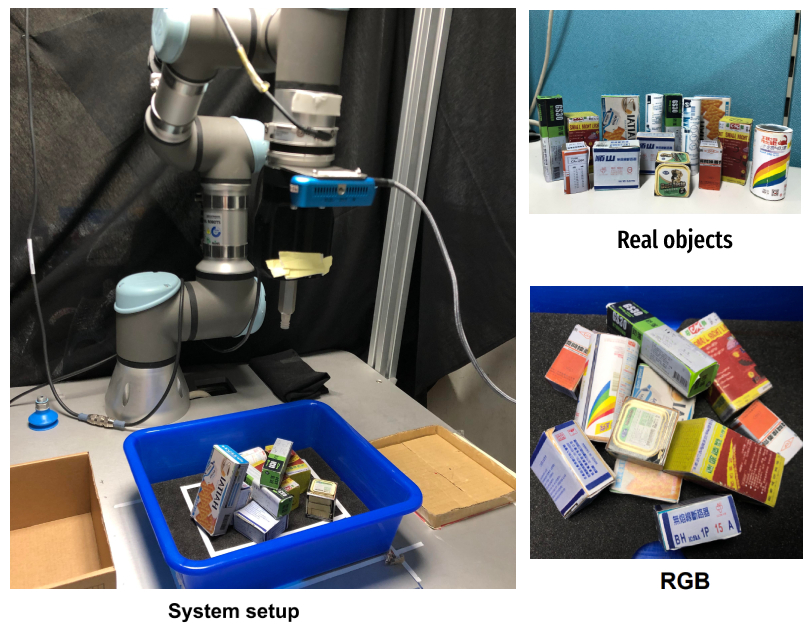}
  \caption{The real picking system setup, the real objects used in the experiment, and sample of observation. We use a UR-3 robot arm with a suction pad.}
  \label{fig:real_env_demo}
\end{center}  
\end{figure}
\end{comment}

\begin{figure}[H]
    \centering
    \begin{subfigure}{0.45\columnwidth}
        \centering
         \includegraphics[width=0.99\columnwidth]{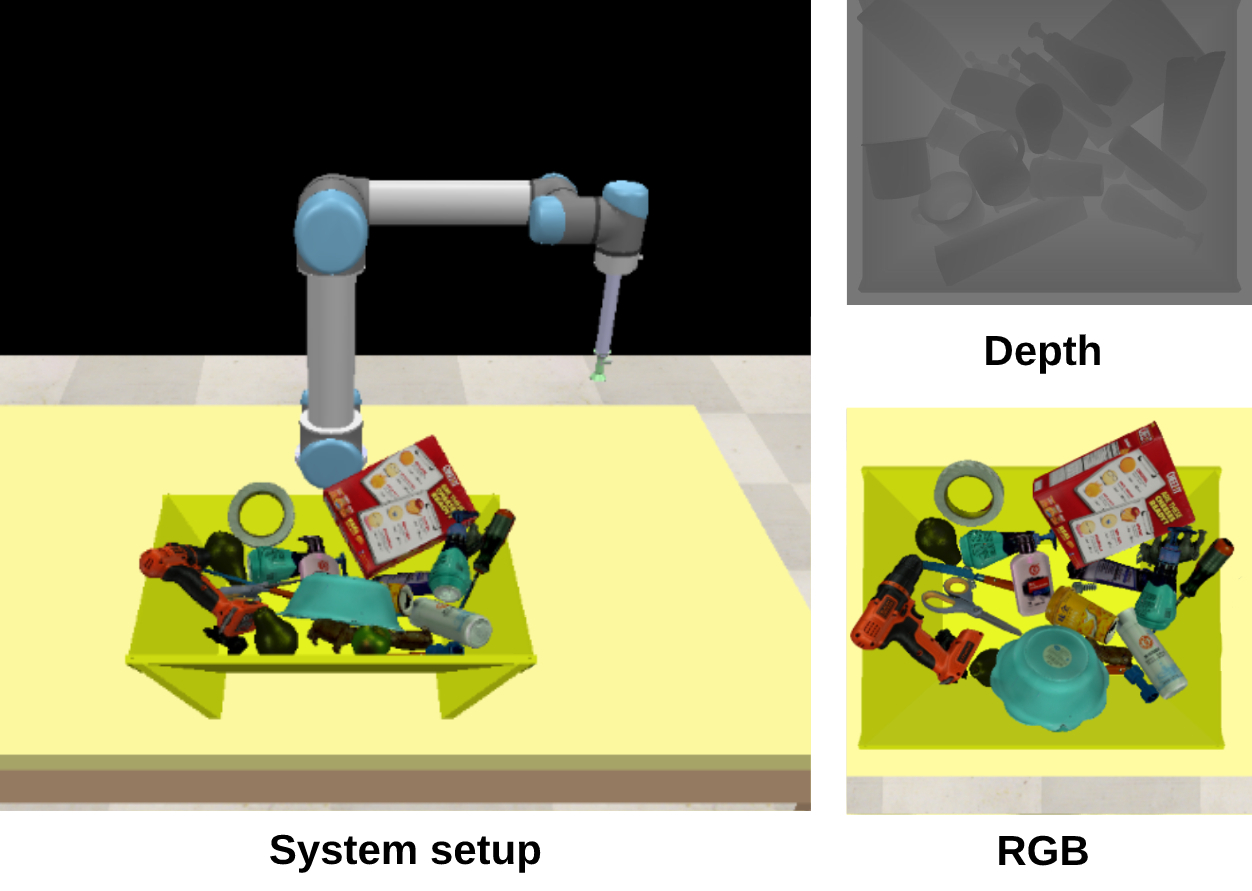}
        \caption{}
        \label{fig:sim_env_demo}
    \end{subfigure}
    \begin{subfigure}{0.41\columnwidth}
        \centering
        \includegraphics[width=0.99\columnwidth]{Materials/real_grasping_setup.jpg}
        \caption{}
        \label{fig:real_env_demo}
    \end{subfigure}
    \caption{(a) The simulation picking system setup, and sample RGB and depth images. We use a UR-5 robot arm with a suction pad gripper. (b) The real picking system setup, the real objects used in the experiment, and sample of observation. We use a UR-3 robot arm with a suction pad.}
    %\label{fig:sup_grasping_result}
\end{figure}
